# Supplementary material for: Automated Proof of Polynomial Inequalities via Reinforcement Learning
Source: arXiv:2503.06592 source file (2025-03-09)
Supplement: Supplementary file 1 [file X_suppl.tex]

\clearpage
\setcounter{page}{1}
\maketitlesupplementary

% \section{Rationale}
% \label{sec:rationale}
% % 
% Having the supplementary compiled together with the main paper means that:
% % 
% \begin{itemize}
% \item The supplementary can back-reference sections of the main paper, for example, we can refer to \cref{sec:intro};
% \item The main paper can forward reference sub-sections within the supplementary explicitly (e.g. referring to a particular experiment); 
% \item When submitted to arXiv, the supplementary will already included at the end of the paper.
% \end{itemize}
% % 
% To split the supplementary pages from the main paper, you can use \href{https://support.apple.com/en-ca/guide/preview/prvw11793/mac#:~:text=Delete%20a%20page%20from%20a,or%20choose%20Edit%20%3E%20Delete).}{Preview (on macOS)}, \href{https://www.adobe.com/acrobat/how-to/delete-pages-from-pdf.html#:~:text=Choose%20%E2%80%9CTools%E2%80%9D%20%3E%20%E2%80%9COrganize,or%20pages%20from%20the%20file.}{Adobe Acrobat} (on all OSs), as well as \href{https://superuser.com/questions/517986/is-it-possible-to-delete-some-pages-of-a-pdf-document}{command line tools}.
\section{Appendix}
\subsection{An Example of LP Transformation}
We provide a simple example to illustrate the transformation process of the polynomial optimization problem into a linear programming problem. \\
%\begin{example}

Consider the polynomial $f(x_1,x_2)=1-5x_1+3x_1x_2-x_1^2+2x_2^2$ with $x_1,x_2\in [0,1]$, and the degree bound $D=2$.
The optimization problem (\ref{opt:orig}) transforms into a linear programming problem as follows:

First, the left-hand side of the equality constraint in (\ref{opt:orig}) can be linearized as 
$f(x_1,x_2)-\gamma={\tilde{{\bf c}}}^{T}{\bf v}$,
where 
$\tilde{{\bf c}}=[1-\gamma,-5,0,1,3,2]^{T}$, and ${\bf v}=[1,x_1,x_2,x_1^2,x_1x_2,x_2^2]^T$.
Similarly, the right-hand side of the equality can be linearized as
$$\sum_{|\alpha|+|\beta|\leq 2}\lambda_{\alpha,\beta}{\bf x}^{\alpha}(1-{\bf x})^{\beta}= {\bf e}^{T}\cdot {\bf v} $$
where ${\bf e}=[e_0,e_1,e_2,e_3,e_4,e_5]^{T}$,
\begin{equation}
\begin{array}{ll}
e_0=\lambda_0+\lambda_2+\lambda_4+\lambda_9,\\ e_1=\lambda_1-\lambda_2+\lambda_5+\lambda_7-\lambda_9,\\
e_2=\lambda_3-\lambda_4+\lambda_8-\lambda_9+\lambda_{10},\\
e_3=-\lambda_5,\\
e_4=\lambda_6-\lambda_7-\lambda_8+\lambda_9,\\\nonumber
e_5=-\lambda_{10}\\
\end{array}
\end{equation}

According to the equality constraint in (\ref{opt:orig}), we can obtain a linear programming problem 
%in the form of Eq.(\ref{opt:matrix}) with variables $\gamma$ and $\lambda$,
whith ${\bf y}=[\gamma,\lambda_0,\ldots,\lambda_{10}]^{T}$, ${\bf c}=[1,-5,0,1,3,2]^{T}$, and matrix
{\small
\begin{equation}
%\scriptsize
\setlength{\arraycolsep}{0.8ex}
A= \left[ {\begin{array}{*{20}{c}}
 1 &1 &0 &1  &0 &1 &0 &0 &0 &0 &1  &0\\ \nonumber
 0 &0 &1 &-1 &0 &0 &1 &0 &1 &0 &-1 &0 \\
 0 &0 &0 &0 &1 &-1 &0 &0 &0 &1 &-1 &1\\
 0 &0 &0 &0 &0 &0 &-1 &0 &0 &0 &0  &0\\
 0 &0 &0 &0 &0 &0 &0  &1 &-1 &-1 &1 &0\\
 0 &0 &0 &0 &0 &0 &0 &0 &0 &0 &0 &-1 
 \end{array}} \right].
 \end{equation}}
 %\end{example}

%%%%%%%%%%%%%%%%%%%%%%%%%%%%%%%%%%%%%%%%%%%%%%%%%%%%%%%%%%%%%%%%%%%%%%%%%%%%%%%%%%%%%%%%%%%%%%%%%%%%%%%%%%%%%%
\subsection{Fast Computation details}
Given the property that a polynomial $h(z)=\sum_{i=0}^{n-1}u_iz^{n-1}$ of degree $n-1$ can be uniquely determined by its value at any $n$ distinct points, we can express the coefficient representation in terms of these points. Let $\omega_n$ be a primitive $n$-th root of 1, i.e., $\omega_n^n=1$, where $\omega_n=\exp{(\frac{-i2\pi}{n})}$ in the complex number field $\mathbb{C}$. The vector ${\bf w}_n=(\omega_n^0,\omega_n^1,\ldots,\omega_n^{n-1})$ contains all the $n$-th roots of 1. Suppose $n=2^{\theta}$, where $\theta$ is a positive integer. We can then decompose $\tilde{p}(z)$ as follows:
\begin{equation}
\left.\begin{array}{l}
h(z)=h_0(\phi)+zh_1(\phi), \vspace{1ex}\\ \nonumber
h_0(\phi)=u_0+u_2\phi+\cdots+u_{n-2}\phi^{\frac{n}{2}-1}, \vspace{1ex}\\
h_1(\phi)=u_1+u_3\phi+\cdots+u_{n-1}\phi^{\frac{n}{2}-1}
\end{array}\right\}
\end{equation}
where $\phi=z^2$. This decomposition reduces the discrete Fourier Transform (DFT) for $h(z)$ to two problems of $DFT_{\frac{n}{2}}$, with an additional step of multiplying $h_1(\phi)$ by $z$  for $z=\omega^j$, $j=0,1,\ldots,n-1$, and pairwise adding the $n$ output values to $h_0(\omega^{2j})$. The DFT is thus defined by:
\begin{equation}\label{eq:DFT}
H_j=\sum_{k=0}^{n-1}u_k\omega_{n}^{jk}=\sum_{k=0}^{n-1}u_ke^{-i2\pi\frac{jk}{n}},
\end{equation}
where $e$ is the base of the natural logarithm, and $i$ is the imaginary unit. The inverse discrete Fourier transform (IDFT) is defined as:
\begin{equation}\label{eq:IDFT}
u_k=\frac{1}{n}\sum_{j=0}^{n-1}H_j\cdot e^{i2\pi\frac{jk}{n}}.
\end{equation}

%%%%%%%%%%%%%%%%%%%%%%%%%%%%%%%%%%%%%%%%%%%%%%%%%%%%
\begin{example}
Given two polynomials $p(x_1,x_2)=x_1+3x_1x_2$, $q(x_1,x_2)=2x_2-5x_1^2$, we aim to compute $p({\bf x})\cdot q({\bf x})$.Both polynomials $p$ and $q$ have a degree of 2. Then we set the upper bound $D = 2\times 2 + 1 = 5$. The polynomial $p$ consists
of two monomials: $x_1$ (with exponent tuples $(1, 0)$) and $x_1x_2$ (with exponent $(1, 1)$).
Thus, we have $\nu_1 = 1 + 0 \times D$ and $\nu_2 = 1 + 1 \times D$. Therefore, the univariate polynomial $\tilde{p}(z)$ obtained is $\tilde{p}(z) = z + 3z^6$.
Similarly, $q$ is transformed into $\tilde{q}(z) = 2z^5-5z^2$.

Next, we compute the univariate polynomial $g(z)$ using FFT, yielding $g(z) = -5z^3 + 2z^6 - 15z^8 + 6z^{11}$. Finally, for each term in $g(z)$, we need to map the univariate exponents using Eq.(\ref{eq:CRT}). 
For example, for the term $z^{11}$, we have $\mu_{1_4} = 11 \mod 5 = 1$ and $\mu_{2_4} = (11 - 1) / 5 \mod 5 = 2$. Thus, $z^{11}$ corresponds to the monomial $x_1x_2^2$. Repeating this for all terms, we obtain the final product in multivariate form:
$p({\bf x})\cdot q({\bf x})=-5x_1^3+2x_1x_2-15x_1^3x_2+6x_1x_2^2.$  $\hfill\square$
\end{example}

\subsection{Experimental details}
%We will now show the details of our experimental part. We implemented a tool called APPIRL in Python based on our framework. You can find it at this URL: https://anonymous.4open.science/r/APPIRL. 

%For all examples in our experiment, the hyperparameters used during training and the trained Q value network model in DQN are also shown in the tool. 
%Next, we will show the polynomials in the experiment.
%We will show the proof process of inequalities with proof steps less than or equal to 20. (We output the actions selected at each step.) 
%For inequalities with proof steps greater than 20, we provide an interface in the APPIRL tool to reproduce the proof process using our trained Q-value neural network model.

We will now show the specifics of the experimental portion. Our algorithm's framework has been implemented in Python, resulting in a tool called APPIRL, which is accessible at 
https://anonymous.4open.science/r/APPIRL. 

For all examples within our experiments, the hyperparameters used during DQN training and the model of the Q-value network are showcased within the toolkit. 
To conserve space, we present the proof process of polynomial inequalities with fewer proof steps (i.e., outputting the action selected at each step). For examples with a larger number of proof steps, we provide an interface within the APPIRL tool that allows for reproduction using the trained Q-value neural network model.

\textbf{{\bf $C_1$:} Mickey-mouse example as illustration}
{\small
\begin{align*}
f(\mathbf{z})=-z_{1} + 2z_{2}^{2} + 1.67 \geq 0
\end{align*}
}
with a hyperrectangle $\mathcal {S}= \{ { \bf z}\in \mathbb{R}^2|z_i\in [-1,1],i=1,\ldots,2 \}$.
After regularizing the variable $\mathbf{z}$, we can obtain
{\small
\begin{align*}
f(\mathbf{x})=-2x_{1} + 8x_{2}^{2} - 8x_{2} + \frac{14}{3} \geq 0
\end{align*}
}
with a unit hypercube $\mathcal{S} = \{ { \bf x}\in [0, 1]^{2}\}$.

{Proof process}:

\textrm{[step 1]} $-x_{2}^{3} + 3*x_{2}^{2} - 3*x_{2} + 1$

\textrm{[step 2]} $-x_{2}^{3} + 3*x_{2}^{2} - 3*x_{2} + 1$

\textrm{[step 3]} $x_{1}*x_{2}^{2}$

\textrm{[step 4]} $-x_{1}^{2}*x_{2} + x_{1}*x_{2}$

\textrm{[step 5]} $x_{1}^{3} - 2*x_{1}^{2} + x_{1}$

\textrm{[step 6]} $x_{1}^{2}*x_{2} - x_{1}^{2} - x_{1}*x_{2} + x_{1}$

\textrm{[step 7]} $x_{2}^{3}$

{ Non-negative representation:}

$2*(1-x_1) + \frac{8}{3}*\textrm{[step 2]} + \frac{8}{3}*\textrm{[step 7]} \geq 0$

\textbf{$C_2$: Mickey-mouse example as illustration}
{\small
\begin{align*}
f(\mathbf{z})=z_{1}^{2} + 4z_{2}^{2} + 1.67 \geq 0
\end{align*}
}
with a hyperrectangle $\mathcal {S}= \{ { \bf z}\in \mathbb{R}^2|z_i\in [-1,1],i=1,\ldots,2 \}$.
After regularizing the variable $\mathbf{z}$, we can obtain:
{\small
\begin{align*}
f(\mathbf{x})=4x_{1}^{2} - 4x_{1} + 16x_{2}^{2} - 16x_{2} + \frac{20}{3} \geq 0
\end{align*}
}
with a unit hypercube $\mathcal{S} = \{ { \bf x}\in [0, 1]^{2}\}$.

{Proof process}:

\textrm{[step 1]} $-x_{1}^{2}*x_{2} + x_{1}^{2}$

\textrm{[step 2]} $-x_{1}^{2}*x_{2} + x_{1}*x_{2}$

\textrm{[step 3]} $-x_{1}*x_{2}^{2} + x_{1}*x_{2}$

\textrm{[step 4]} $-x_{1}^{2}*x_{2} + x_{1}*x_{2}$

\textrm{[step 5]} $-x_{1}^{3} + 3*x_{1}^{2} - 3*x_{1} + 1$

\textrm{[step 6]} $-x_{1}*x_{2}^{2} + 2*x_{1}*x_{2} - x_{1} + x_{2}^{2} - 2*x_{2} + 1$

\textrm{[step 7]} $-x_{2}^{3} + 3*x_{2}^{2} - 3*x_{2} + 1$

\textrm{[step 8]} $-x_{1}*x_{2}^{2} + x_{1}*x_{2}$

\textrm{[step 9]} $x_{1}^{2}*x_{2} - x_{1}^{2} - x_{1}*x_{2} + x_{1}$

\textrm{[step 10]} $x_{1}^{3} - 2*x_{1}^{2} + x_{1}$

\textrm{[step 11]} $x_{1}^{2}*x_{2} - x_{1}^{2} - x_{1}*x_{2} + x_{1}$

\textrm{[step 12]} $x_{1}*x_{2}^{2} - 2*x_{1}*x_{2} + x_{1}$

\textrm{[step 13]} $x_{1}*x_{2}^{2} - 2*x_{1}*x_{2} + x_{1}$

\textrm{[step 14]} $x_{2}^{3}$

\textrm{[step 15]} $-x_{2}^{3} + 3*x_{2}^{2} - 3*x_{2} + 1$

\textrm{[step 16]} $-x_{1}^{3} + x_{1}^{2}$

\textrm{[step 17]} $x_{1}^{2}*x_{2}$

\textrm{[step 18]} $x_{1}^{2}*x_{2}$

\textrm{[step 19]} $x_{1}^{3}$

{ Non-negative representation:}

{\small
\begin{align*}
&\frac{4}{3}*\textrm{[step 5]}+\frac{16}{3}*\textrm{[step 15]} +\frac{16}{3}*\textrm{[step 14]}+\\
&\frac{4}{3}*\textrm{[step 19]} \geq 0
\end{align*}}

\textbf{$C_3$: A 3-dimensional reaction diffusion problem}
{\small
\begin{align*}
&f(\mathbf{z})=-z_{1} + 0.835634534z_{2}^{2} + 1.164365466z_{2} \\
&\quad\quad-z_{3} + 18.904230228 \geq 0
\end{align*}
}
with a hyperrectangle $\mathcal {S}= \{ { \bf z}\in \mathbb{R}^3|z_i\in [-5,5],i=1,\ldots,3 \}$.
After regularizing the variable $\mathbf{z}$, we can obtain
{\small
\begin{align*}
&f(\mathbf{x})=-10x_{1} + 83.5634534x_{2}^{2} - 71.91979874x_{2} \\
&\quad\quad-10x_{3} + 43.973266248 \geq 0
\end{align*}
}
with a unit hypercube $\mathcal{S} = \{ { \bf x}\in [0, 1]^{3}\}$.

{Proof process}:

\textrm{[step 1]} $-x_{1}*x_{2}^{2} + x_{2}^{2}$

\textrm{[step 2]} $x_{2}*x_{3}^{2}$

\textrm{[step 3]} $-x_{1}*x_{2}*x_{3} + x_{2}*x_{3}$

\textrm{[step 4]} $-x_{2}^{2}*x_{3} + x_{2}*x_{3}$

\textrm{[step 5]} $x_{2}^{3} - 2*x_{2}^{2} + x_{2}$

\textrm{[step 6]} $x_{1}^{3} - 2*x_{1}^{2} + x_{1}$

\textrm{[step 7]} $x_{1}*x_{2}^{2} - 2*x_{1}*x_{2} + x_{1}$

\textrm{[step 8]} $x_{2}^{3}$

\textrm{[step 9]} $-x_{2}^{3} + x_{2}^{2}$

\textrm{[step 10]} $-x_{2}^{2}*x_{3} + x_{2}^{2}$

\textrm{[step 11]} $x_{2}*x_{3}^{2}$

\textrm{[step 12]} $-x_{1}*x_{2}*x_{3} + x_{2}*x_{3}$

\textrm{[step 13]} $-x_{2}^{2}*x_{3} + x_{2}*x_{3}$

\textrm{[step 14]} $x_{1}*x_{2}*x_{3} - x_{1}*x_{2} - x_{2}*x_{3} + x_{2}$

\textrm{[step 15]} $x_{1}^{2}*x_{3} - 2*x_{1}*x_{3} + x_{3}$

\textrm{[step 16]} $-x_{1}*x_{2}*x_{3} + x_{1}*x_{2} + x_{1}*x_{3} - x_{1} + x_{2}*x_{3} - x_{2} - x_{3} + 1$

\textrm{[step 17]} $-x_{2}^{3} + 3*x_{2}^{2} - 3*x_{2} + 1$

{Non-negative representation:}
\begin{equation*}
\begin{array}{ll}
&10*(1-x_1)+10*(1-x3)+35.61692091*\\
&\textrm{[step 8]} + 11.64365466*\textrm{[step 9]}+\\
&23.97326625*\textrm{[step 17]} \geq 0
\end{array}
\end{equation*}

\textbf{$C_4$: A neural network modeled by an adaptive Lotka-Volterra system}
{\small
\begin{align*}
f(\mathbf{z})=z_{1}z_{2}^{2} + z_{1}z_{3}^{2} - 1.1z_{1} + 10.35 \geq 0
\end{align*}
}
with a hyperrectangle $\mathcal {S}= \{ { \bf z}\in \mathbb{R}^3|z_i\in [-1.5,2],i=1,\ldots,3 \}$.
After regularizing the variable $\mathbf{z}$, we can obtain
{\small
\begin{align*}
&f(\mathbf{x})=42.875x_{1}x_{2}^{2} - 36.75x_{1}x_{2} + 42.875x_{1}x_{3}^{2} -
36.75x_{1}x_{3} \\
&\quad\quad+ 11.9x_{1} - 18.375x_{2}^{2} + 15.75x_{2}-18.375x_{3}^{2} + 15.75x_{3}\\
&\quad\quad + 5.25 \geq 0
\end{align*}
}
with a unit hypercube $\mathcal{S} = \{ { \bf x}\in [0, 1]^{3}\}$. 
%The proof process requires ?? steps.

\textbf{$C_5$: A neural network modeled by an adaptive Lotka-Volterra system}
{\small
\begin{align*}
f(\mathbf{z})=z_{1}z_{2}^{2} + z_{1}z_{3}^{2} + z_{1}z_{4}^{2} - 1.1z_{1} + 21.8 \geq 0
\end{align*}
}
with a hyperrectangle $\mathcal {S}= \{ { \bf z}\in \mathbb{R}^4|z_i\in [-2,2],i=1,\ldots,4 \}$.
After regularizing the variable $\mathbf{z}$, we can obtain
{\small
\begin{align*}
&f(\mathbf{x})=64x_{1}x_{2}^{2} - 64x_{1}x_{2} + 64x_{1}x_{3}^{2} - 64x_{1}x_{3} + 64x_{1}x_{4}^{2} \\
&\quad\quad-64x_{1}x_{4} + 43.6x_{1} - 32x_{2}^{2} + 32x_{2} - 32x_{3}^{2} + 32x_{3} \\
&\quad\quad-32x_{4}^{2} + 32x_{4} \geq 0
\end{align*}
}
with a unit hypercube $\mathcal{S} = \{ { \bf x}\in [0, 1]^{4}\}$.

{Proof process}:

\textrm{[step 1]} $-x_{1}*x_{2}*x_{3}^{2} + x_{1}*x_{3}^{2}$

\textrm{[step 2]} $-x_{1}*x_{3}^{3} + 3*x_{1}*x_{3}^{2} - 3*x_{1}*x_{3} + x_{1}$

\textrm{[step 3]} $-x_{1}^{2}*x_{2}*x_{4} + x_{1}^{2}*x_{2} + x_{1}^{2}*x_{4} - x_{1}^{2} + x_{1}*x_{2}*x_{4} - x_{1}*x_{2} - x_{1}*x_{4} + x_{1}$

\textrm{[step 4]} $-x_{1}^{2}*x_{2}*x_{3} + x_{1}^{2}*x_{2} + x_{1}^{2}*x_{3} - x_{1}^{2} + x_{1}*x_{2}*x_{3} - x_{1}*x_{2} - x_{1}*x_{3} + x_{1}$

\textrm{[step 5]} $-x_{1}^{2}*x_{3}*x_{4} + x_{1}^{2}*x_{3} + x_{1}^{2}*x_{4} - x_{1}^{2} + x_{1}*x_{3}*x_{4} - x_{1}*x_{3} - x_{1}*x_{4} + x_{1}$

\textrm{[step 6]} $-x_{1}*x_{2}*x_{3}*x_{4} + x_{1}*x_{2}*x_{3} + x_{1}*x_{2}*x_{4} - x_{1}*x_{2} + x_{1}*x_{3}*x_{4} - x_{1}*x_{3} - x_{1}*x_{4} + x_{1}$

\textrm{[step 7]} $-x_{1}*x_{4}^{3} + 3*x_{1}*x_{4}^{2} - 3*x_{1}*x_{4} + x_{1}$

\textrm{[step 8]} $x_{1}*x_{3}^{3}$

{Non-negative representation:}
\begin{equation*}
\begin{array}{ll}
&\frac{28}{15}*(-x_2^2 + x_2) + \frac{254}{15}*x1*x_2^2+ 16 * x_1*x_4^2 + \vspace{1ex}\\
&\frac{254}{15}*(x_1*x_2^2 - 2*x_1*x_2 + x_1)+ 16 *(x_1*x_4^2 -\vspace{1ex}\\
&2*x_1*x_4+ x_1)+\frac{452}{15}*(x_1*x_2^2 - x_1*x_2 - x_2^2 + x_2)\vspace{1ex}\\
&+32*(x_1*x_3^2 - x_1*x_3 - x_3^2 + x_3)+ 32*(x_1*x_4^2 \vspace{1ex}\\
&- x_1*x_4 - x_4^2 + x_4) + \frac{32}{3}*\textrm{[step 2]}+ \frac{32}{3}*\textrm{[step 8]} \geq 0
\end{array}
\end{equation*}

% $\frac{28}{15}*(-x_2^2 + x_2) + \frac{254}{15}*x1*x_2^2+ 16 * x_1*x_4^2 +\frac{254}{15}*(x_1*x_2^2 - 2*x_1*x_2 + x_1)+ 16 *(x_1*x_4^2 - 2*x_1*x_4+ x_1)+\frac{452}{15}*(x_1*x_2^2 - x_1*x_2 - x_2^2 + x_2)+32*(x_1*x_3^2 - x_1*x_3 - x_3^2 + x_3)+ 32*(x_1*x_4^2 - x_1*x_4 - x_4^2 + x_4) + \frac{32}{3}*\textrm{[step 2]}+ \frac{32}{3}*\textrm{[step 8]} \geq 0$

\textbf{$C_6$: A neural network modeled by an adaptive Lotka-Volterra system}
{\small
\begin{align*}
f(\mathbf{z})=-z_{1}z_{2}^{2} - z_{1}z_{3}^{2} - z_{1}z_{4}^{2} + 1.1z_{1} + 21.8 \geq 0
\end{align*}
}
with a hyperrectangle $\mathcal {S}= \{ { \bf z}\in \mathbb{R}^4|z_i\in [-2,2],i=1,\ldots,4 \}$.
After regularizing the variable $\mathbf{z}$, we can obtain
{\small
\begin{align*}
&f(\mathbf{x})=-64x_{1}x_{2}^{2} + 64x_{1}x_{2} - 64x_{1}x_{3}^{2} + 64x_{1}x_{3} - 64x_{1}x_{4}^{2} \\
&\quad\quad+64x_{1}x_{4} - 43.6x_{1} + 32x_{2}^{2} - 32x_{2} + 32x_{3}^{2} - 32x_{3} +\\
&\quad\quad+32x_{4}^{2} - 32x_{4} + 43.6 \geq 0
\end{align*}
}
with a unit hypercube $\mathcal{S} = \{ { \bf x}\in [0, 1]^{4}\}$.

\textbf{$C_7$:Caprasse’s system}
{\small
\begin{align*}
&f(\mathbf{z})=z_{1}z_{3}^{3} - 4z_{1}z_{3}z_{4}^{2} - 4z_{1}z_{3} - 4z_{2}z_{3}^{2}z_{4} - 2z_{2}z_{4}^{3} \\
&\quad\quad+10z_{2}z_{4} - 4z_{3}^{2} + 10z_{4}^{2} + 5325 \geq 0
\end{align*}
}
with a hyperrectangle $\mathcal {S}= \{ { \bf z}\in \mathbb{R}^4|z_i\in [-5,5],i=1,\ldots,4 \}$.
After regularizing the variable $\mathbf{z}$, we can obtain
{\small
\begin{align*}
&f(\mathbf{x})=10000x_{1}x_{3}^{3} - 15000x_{1}x_{3}^{2} - 40000x_{1}x_{3}x_{4}^{2} \\
&\quad\quad+40000x_{1}x_{3}x_{4} - 2900x_{1}x_{3} + 20000x_{1}x_{4}^{2} \\
&\quad\quad-20000x_{1}x_{4} + 3950x_{1} - 40000x_{2}x_{3}^{2}x_{4}  \\
&\quad\quad+20000x_{2}x_{3}^{2} + 40000x_{2}x_{3}x_{4} - 20000x_{2}x_{3} \\
&\quad\quad-20000x_{2}x_{4}^{3} + 30000x_{2}x_{4}^{2} - 24000x_{2}x_{4} \\
&\quad\quad+7000x_{2} - 5000x_{3}^{3} + 20000x_{3}^{2}x_{4} - 2900x_{3}^{2} \\
&\quad\quad+20000x_{3}x_{4}^{2} - 40000x_{3}x_{4} + 11850x_{3} \\
&\quad\quad+10000x_{4}^{3} - 24000x_{4}^{2} + 21000x_{4} \geq 0
\end{align*}
}
with a unit hypercube $\mathcal{S} = \{ { \bf x}\in [0, 1]^{4}\}$.

\textbf{$C_8$: System of A. H. Wright}
{\small
\begin{align*}
f(\mathbf{z})=z_{1} + z_{2} + z_{3} + z_{4} + z_{5}^{2} - z_{5} + 30 \geq 0
\end{align*}
}
with a hyperrectangle $\mathcal {S}= \{ { \bf z}\in \mathbb{R}^5|z_i\in [-5,5],i=1,\ldots,5 \}$.
After regularizing the variable $\mathbf{z}$, we can obtain
{\small
\begin{align*}
f(\mathbf{x})=&10x_{1} + 10x_{2} + 10x_{3} + 10x_{4} + \\
&100x_{5}^{2} - 110x_{5} + 40 \geq 0
\end{align*}
}
with a unit hypercube $\mathcal{S} = \{ { \bf x}\in [0, 1]^{5}\}$.

{Proof process}:

\textrm{[step 1]} $x_{2}*x_{4}*x_{5} - x_{2}*x_{5} - x_{4}*x_{5} + x_{5}$

\textrm{[step 2]} $x_{5}^{3}$

\textrm{[step 3]} $-x_{5}^{3} + 3*x_{5}^{2} - 3*x_{5} + 1$

{ Non-negative representation:}
\begin{equation*}
\begin{array}{ll}
&20*x_1*x_2+10*x_1*x_3+10*x_1*x_4+\\
&10*x_1*(1-x_2) +10*x_2*(1-x_1)+\\
&10*x_3*(1-x_1)+10*x_4*(1-x_1)\\
&+10*(1-x_5)^2+30*\textrm{[step 2]}+30*\textrm{[step 3]} \geq 0
\end{array}
\end{equation*}

\textbf{$C_9$:The cyclic 5-roots problem}
{\small
\begin{align*}
&f(\mathbf{z})=z_{1}z_{2}z_{3}z_{4} + z_{1}z_{2}z_{3}z_{5} + z_{1}z_{2}z_{4}z_{5} +z_{1}z_{3}z_{4}z_{5} \\
&\quad\quad+z_{2}z_{3}z_{4}z_{5} + 30000 \geq 0
\end{align*}
}
with a hyperrectangle $\mathcal {S}= \{ { \bf z}\in \mathbb{R}^5|z_i\in [-10,10],i=1,\ldots,5 \}$.
After regularizing the variable $\mathbf{z}$, we can obtain
{\small
\begin{align*}
&f(\mathbf{x})=160000x_{1}x_{2}x_{3}x_{4} + 160000x_{1}x_{2}x_{3}x_{5} - 160000x_{1}x_{2}x_{3}\\
&\quad\quad+ 160000x_{1}x_{2}x_{4}x_{5} - 160000x_{1}x_{2}x_{4} - 160000x_{1}x_{2}x_{5}\\
&\quad\quad+ 120000x_{1}x_{2} + 160000x_{1}x_{3}x_{4}x_{5} - 160000x_{1}x_{3}x_{4}\\
&\quad\quad- 160000x_{1}x_{3}x_{5} + 120000x_{1}x_{3} - 160000x_{1}x_{4}x_{5} \\
&\quad\quad+ 120000x_{1}x_{4} + 120000x_{1}x_{5} - 80000x_{1} \\
&\quad\quad+ 160000x_{2}x_{3}x_{4}x_{5} - 160000x_{2}x_{3}x_{4} - 160000x_{2}x_{3}x_{5} \\
&\quad\quad+ 120000x_{2}x_{3} - 160000x_{2}x_{4}x_{5} + 120000x_{2}x_{4}\\
&\quad\quad+ 120000x_{2}x_{5} - 80000x_{2} - 160000x_{3}x_{4}x_{5} \\
&\quad\quad+ 120000x_{3}x_{4} + 120000x_{3}x_{5} - 80000x_{3} \\
&\quad\quad+ 120000x_{4}x_{5} - 80000x_{4} - 80000x_{5} + 80000 \geq 0
\end{align*}
}
with a unit hypercube $\mathcal{S} = \{ { \bf x}\in [0, 1]^{5}\}$.

\textbf{$C_{10}$: Camera displacement between two positions, scaled first frame}
{\small
\begin{align*}
&f(\mathbf{z})=-6.8z_{1}z_{4} - 3.2z_{1}z_{5} + 1.3z_{1}z_{6} + 5.1z_{1} -
4.8z_{2}z_{5} \\
&\quad\quad- 0.7z_{2}z_{6} - 7.1z_{2} - 1.9z_{3}z_{4} - 0.7z_{3}z_{5} + 9z_{3}z_{6} \\
&\quad\quad- z_{3} + 5.1z_{4} - 7.1z_{5} - z_{6} + 270400 \geq 0
\end{align*}
}
with a hyperrectangle $\mathcal {S}= \{ { \bf z}\in \mathbb{R}^6|z_i\in [-100,100],i=1,\ldots,6 \}$.
After regularizing the variable $\mathbf{z}$, we can obtain
{\small
\begin{align*}
&f(\mathbf{x})=-272000x_{1}x_{4} - 128000x_{1}x_{5} + 52000x_{1}x_{6} \\
&\quad\quad+175020x_{1} - 192000x_{2}x_{5} - 28000x_{2}x_{6} \\
&\quad\quad+108580x_{2} - 76000x_{3}x_{4} - 28000x_{3}x_{5} \\
&\quad\quad+360000x_{3}x_{6} - 128200x_{3} + 175020x_{4} \\
&\quad\quad+172580x_{5} - 192200x_{6} + 193000 \geq 0
\end{align*}
}
with a unit hypercube $\mathcal{S} = \{ { \bf x}\in [0, 1]^{6}\}$.
